# Supplementary material for: Distributed Pruning Towards Tiny Neural Networks in Federated Learning
Source: arXiv:2212.01977 source file (2023-07-11)
Supplement: Supplementary file 1 [file appendix.tex]

\subsection{Effect of Progressive Pruning}
We apply a growing-pruning adjustment to the model structure while maintaining the sparsity. Specifically, the server grows the pruned parameters and
prunes the same number of unpruned parameters to adjust the model structure. Like prior works~\cite{janowsky1989pruning, han2015deep}, we prune the parameters with the smallest magnitude. On the one hand, the squared value of weights can be viewed as weight power, and magnitude pruning removes the parameters with the least power to improve the computational efficiency~\cite{hagiwara1993removal}. On the other hand, magnitude pruning can remove trivial parameters and increase the generalization ability of the network. 

After pruning, we grow the pruned parameters with the largest gradient magnitude, like RigL~\cite{evci2020rigging}. If the gradient magnitude of a pruned parameter is large, this parameter is important and should not be pruned. Growing pruned parameters with high gradients will reduce the loss quickly, which can help the model structure to reach optimal faster in Equation~\ref{eq:obj}.

\subsection{The Impact of Pruning Schedule}
The pruning schedule determines the pruning granularity and pruning frequency in the progressive pruning module. For pruning granularity, we choose to prune one layer per round (Layer), pruning one block per round (Block), and prune the entire model per round (Entire). We divide the model into five blocks to prune, as shown in Figure~\ref{fig:grand}. Moreover, we control the pruning frequencies by setting different interval rounds $\Delta R$ between two pruning. Since the pruning times of each layer should be the same, we set corresponding stopping rounds $R_{stop}$ for different pruning granularity and $\Delta R$. Moreover, We also wonder if the order in which layers or blocks are selected to prune has any effect.

\subsection{The Impact of Data Heterogeneity}
Neural network pruning requires training data to determine the proper model structure. Due to resource-constrained devices, the server cannot push the dense model to devices. Therefore, the server needs to coarsely prune to produce the initial pruned model. Due to privacy concerns in federated learning, the server cannot know the data distributions for all clients. So, in the existing methods, the server only coarsely prunes the model based on the pretrain dataset or the data from some trusted clients. It makes the dataset used for pruning different from the dataset used for fine-tuning, which causes bias in coarse pruning. Therefore, our strategy is to use adaptive BN selection to select one pruned model with less bias. 

To show the impact of the data heterogeneity, we set different non-iid degrees by using different $\alpha$ in the Dirichlet distribution. Lower $\alpha$ indicates a higher Non-IID degree. We do experiments on the CIFAR-10 dataset with ResNet18 with 1\% density. The experiments are shown in Figure~\ref{fig:noniid}. Our experiments show that 1) the performance of the existing pruning methods (e.g., SynFlow, LotteryFL) in Federated Learning will be significantly degraded given a higher non-iid degree; 2) Our proposed FedTiny mitigates the bias in pruning and achieves the best performance compared with the existing pruning methods.

\begin{figure}[!tb]
\centering
\includegraphics[width=0.45\columnwidth]{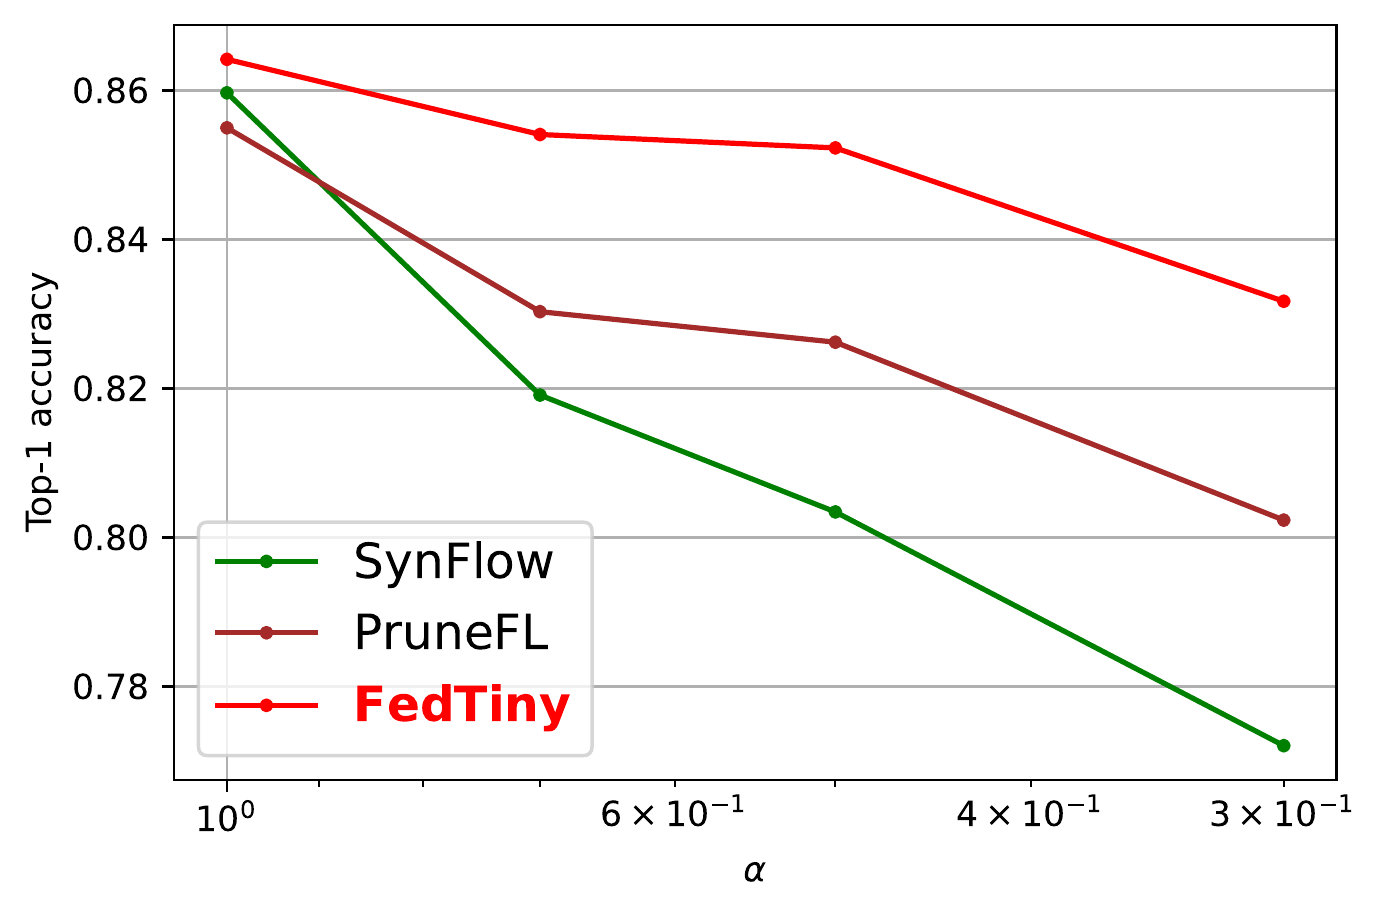} % Reduce the figure size so that it is slightly narrower than the column. Don't use precise values for figure width.This setup will avoid overfull boxes.
\caption{Top-1 accuracy of different pruning approaches on various non-iid degrees. Lower $\alpha$ indicates a higher Non-IID degree.}
\label{fig:noniid}
\vspace{-1em}
\end{figure}

\subsection{The performance of Small Model}

Although FedTiny can outperform other baselines in the very sparse model, like 1\% density, the accuracy suffers from a drop compared to the full-size models. The small model can be considered as a baseline in this case. Therefore, we design the experiments on small models. We train a small network with 3 convolutional layers. First, we evaluate the small network with a similar number of parameters to ResNet18 with 1\% density on different datasets. Second, we evaluate the small network with a similar number of parameters to ResNet18 with different densities on CIFAR-10.
 We also choose SynFlow and LotteryFL as references. The experiment result is shown in Table~\ref{tab:smallcnn1} and Table~\ref{tab:smallcnn2}. The experimental results show that the small network is competitive compared to other baselines. However, our proposed FedTiny achieves much better performance compared with the small network, which demonstrates the advantage of FedTiny.

\begin{table}[]
\centering
\begin{tabular}{l|llll}
\hline
Dataset   & SynFlow & LotteryFL & Small Model    & FedTiny \\ \hline
CIFAR-10  & 0.8034  & 0.8262    & 0.8019 & 0.8523  \\
CINIC-10  & 0.6057  & 0.6379    & 0.5578 & 0.6712  \\
SVHN      & 0.8683  & 0.8927    & 0.8395 & 0.8826  \\
CIFAR-100 & 0.4413  & 0.4373    & 0.4277 & 0.4865  \\ \hline
\end{tabular}
\caption{The Top-1 accuracy for ResNet18 with 1\% density and a small model on a different dataset. }
\label{tab:smallcnn1}
\end{table}

\begin{table}[]
\centering
\begin{tabular}{l|llll}
\hline
Density & SynFlow & LotteryFL & small models   & FedTiny \\ \hline
0.01    & 0.8034  & 0.8262    & 0.8019 & 0.8523  \\
0.005   & 0.7206  & 0.736     & 0.7201 & 0.7972  \\
0.003   & 0.6279  & 0.6453    & 0.6921 & 0.7572  \\
0.001   & 0.2862  & 0.2955    & 0.6158 & 0.6311  \\ \hline
\end{tabular}
\caption{The Top-1 accuracy for ResNet18 with various densities and small models on CIFAR-10 dataset.}
\label{tab:smallcnn2}
\end{table}

\subsection{The Impact of Large Client Number}
\label{app:largenumber}
To evaluate the performance of federated pruning in scenarios with a large number of clients. We conduct federated learning with 100 clients to verify the scalability of our proposed FedTiny. Only 10 clients are selected in each round. On the CIFAR-10 dataset with ResNet18 in 1\% density, after 500 rounds of training, FedTiny gets 71.12\% top-1 accuracy. For other baselines, SynFlow gets 59.25\% accuracy, PruneFL gets 62.08\% accuracy and LotteryFL gets 56.80\% accuracy. FedTiny still achieves the best performance compared with the existing pruning methods.

\subsection{Candidate Pool Generation}
\label{app:perlayer}
Given target density $d_{target}$, server outputs candidates in the form of layer-wise pruning rate vectors $(d^1, d^2, \dots, d^L)$ for $L$-layer model based on Uniform Noise (UN) strategies. We derive the density $d^l$ for the $l$-th layer by adding the target density target with random noise $e^l$, i.e., $d^l =d_{target}+e^l$. A candidate can be added to the candidate pool only if its total density $d$ satisfies $d \le d_{target}$. After that, server can get a candidate pool $ \{\theta^{(1)} , \theta^{(2)},\dots, \theta^{(C)} \}$ with mask $\{m^{(1)}, m^{(2)}, \dots, m^{(C)} \}$

\subsection{The Performance of EfficientNet}
\label{app:effi}
Since we focus on specialized tiny models, we evaluate the proposed FedTiny on EfficientNet\cite{tan2019efficientnet}, which is a state-of-the-art neural network model for small devices. We conduct the experiments on CINIC-10 and set the density as 1\%. As shown in the table~\ref{tab:efficientNet}, FedTiny largely outperforms the existing methods (SynFlow, PruneFL, LotteryFL), which is similar to the result in our paper. The experimental results suggest our proposed FedTiny can be generalized to different models and outperforms the existing methods.

\begin{table}[]
\centering
\begin{tabular}{lllll}
\hline
Full-size & SynFlow & PruneFL & LotteryFL   & FedTiny \\ \hline
0.725    & 0.6546  & 0.6809    & 0.6661 & 0.7096 \\ \hline
\end{tabular}
\caption{Top-1 accuracy for EfficientNet with 1\% density on CINIC-10 dataset.}
\label{tab:efficientNet}
\end{table}

\subsection{Calculating FLOPs and Memory for Models}
\label{app:A}
\subsubsection{Compression Schemes} 
\label{app:compression}
The storage for a matrix contains two parts, value, and position. And compression goal is to reduce the storage of the positions of non-zero values in the matrix. Assuming we want to store the positions of $m$ non-zeros value with $b$ bit-width in a sparse matrix $M$. Matrix $M$ has $n$ elements and $n_r \times n_c$ shape. For different densities $d = m/n$, we apply different schemes to represent matrix $M$. We use $o$ bits to represent the position of $m$ non-zeros value and denote the overall storage as $s$. 
\begin{itemize}
    \item For density $d \in [0.9, 1]$, \textbf{dense} scheme is applied, i.e. $s = n * b$.
    \item For density $d \in [0.3, 0.9)$, \textbf{bitmap} (BM) is applied, which stores a map with $n$ bits, i.e. $o = n, s = o + mb$.
    \item For density $d \in [0.1, 0.3)$, we apply \textbf{coordinate offset} (COO), which stores elements with its absolute offset and it requires $o = m  \lceil\log_2n \rceil$ extra bits to store position. Therefore, the overall storage is $s = o + mb$
    \item For density $d \in [0., 0.1)$, we apply \textbf{compressed sparse row} (CSR) and \textbf{compressed sparse column} (CSC) depending on size. It uses column and row index to store the position of elements and $o = m\lceil \log_2 n_c \rceil + n_r\lceil \log_2m\rceil$ bits are needed for CSR. The overall storage is $s = o + mb$
\end{itemize}

For tenor, we only compress the two dimensions with the highest length. With the above strategy, we can further calculate the storage and memory of the parameters in the network. 

\subsubsection{Storage of Model} 
For each tensor or matrix parameter in the model, we identify its density and use the corresponding compression scheme~\ref{app:compression} to represent it. The storage for hyper-parameters is omitted since it is negligible.

\subsubsection{The Memory Footprint of Training Models} 
We estimate training memory footprint as the combination of parameters, activations, gradients of activations, and gradients of parameters. The memory of parameters is equal to the storage of parameters. And we estimate the memory of activation by taking the maximum value of multiple measurements. For simplicity, we set the memory of gradients of activations to be equal to the memory of activations. We omit the memory of hyper-parameters and momentum. Assuming the memory for dense and sparse parameters are $M^p_d$ and $M^p_s$ respectively, and the memory for activations is $M^a$, the overall training memory for each algorithm would be the following:
\begin{itemize}
    \item \textbf{FedAvg and LotteryFL} These methods need to train a dense model, so the memory for gradients of parameters is approximate to $M^p_d$. The training memory footprint is about $2M^p_d + 2M^a$.
    \item \textbf{FL-PQSU, SNIP, and SynFlow} These methods train a sparse static model, so the memory for gradients of parameters is approximate to $M^p_s$. The training memory footprint is about $2M^p_s + 2M^a$.
    \item \textbf{PruneFL}  It requires clients to maintain dense gradients for the full-size parameters, so the memory for gradients of parameters is approximate to $M^p_d$. the memory footprint is about $ M^p_d + M^p_s + 2M^a$.
    \item \textbf{FedTiny.}  Since we divide the model into 5 blocks and adjust one block in one round. Moreover, we only update top-K gradients in memory to adjust model structure, so the extra memory is used to store top-$a^t_l$ gradients and their indices in one block. So the memory for gradients of parameters is approximate to $M^p_s + 3b\sum_l a^t_l$, where $b$ is the bit-width.
    So the overall memory footprint is $2M^p_s + 2M^a + 3b\sum_l a^t_l$. Since the $3b\sum_l a^t_l$ is too small, the overall training memory footprints in FedTiny are approximate to FL-PQSU, SNIP, and SynFlow.
\end{itemize}

\subsubsection{FLOPs of Training Models} 
The training FLOPs include forward pass FLOPs and backward pass FLOPs. We count the total number of operations layer by layer. In the forward pass, the layer activations are computed sequentially using the previous activations and the layer's parameters. And in the backward pass, each layer computes the activation gradient and the gradient of parameters. For simplicity, we default to \textbf{twice} as many FLOPs in the backward pass as in the forward pass. We omit the FLOPs in batch normalization and loss calculation. Assuming the local iteration number is $E$ and the FLOPs for one forward pass with a dense and sparse model are $F_d$ and $F_s$ respectively, the training FLOPs peak in a round on one client is computed as follows:
\begin{itemize}
    \item \textbf{FedAvg and LotteryFL}: These methods need to train the dense model at the beginning. Thus the peak  training FLOPs peak occurs in the first round, which is $3F_dE$.
    \item \textbf{FL-PQSU, SNIP, and SynFlow}: These server-side pruning methods only train static sparse models during the training. Thus, peak training FLOPs are $3F_sE$.
    \item \textbf{PruneFL.} The training FLOPs peak occurs in the adaptive pruning (finer pruning) round, where clients maintain dense gradients for full-size parameters. Thus the backward pass is dense, and the peak FLOPs is $(2F_s + F_d)E$. 
    \item \textbf{FedTiny.} The training FLOPs peak occurs in the finer pruning round.
    Since We divide the model into 5 blocks and prune one block in one round, in the finer pruning round, each client first applies the $E$ epoch of local SGD. Then, the client sample one batch of data to calculate gradients for pruned parameters on the selected block. We find the maximum of extra FLOPs for the selected block is about $0.4F_d$. Therefore, the peak FLOPs of FedTiny is $3F_sE +  0.4F_d$. The ratio of FLOPs peak in FedTiny and FedAvg is $\frac{Fs}{F_d} + \frac{0.4}{3E}$, where the first term is equal to server-side pruning methods. The second term is as small as 0.0004 with our experiment settings. Therefore, the training FLOPs peak in our FedTiny is approximate to the server-side pruning method.
\end{itemize}

% \begin{table}[!tb]
% \renewcommand\arraystretch{1.2} % adjust space between rows
% \centering
% % \resizebox{0.9\linewidth}{!}{
% \begin{tabular}{cc|ccc}
% \hline
% Density &
%   \begin{tabular}[c]{@{}c@{}}Pool\\  Size\end{tabular} &
%   Accuracy &
%   \begin{tabular}[c]{@{}c@{}}Storage \&\\   Communication \end{tabular}\\ \hline
% 1     & 1   & 0.8696 & 515.23MB \\ \hline
% \multicolumn{1}{c}{\multirow{4}{*}{0.01}} &
%   50 & 0.7883 & 468.43MB  \\
% \multicolumn{1}{c}{} &
%   20 & 0.7901 & 187.19MB \\
% \multicolumn{1}{c}{} &
%   10 & 0.7892 & 93.58MB\\
% \multicolumn{1}{c}{} &
%   1  & 0.7537 & 9.37MB\\
% \hline
% \multicolumn{1}{c}{\multirow{4}{*}{0.005}} &
%   50 & 0.7534 & 244.18MB\\
% \multicolumn{1}{c}{} &
%   20 & 0.7495 & 97.41MB  \\
% \multicolumn{1}{c}{} &
%   10 & 0.7409 & 48.74MB\\
% \multicolumn{1}{c}{} &
%   1  & 0.7032 & 4.88MB \\
% \hline
% \multicolumn{1}{c}{\multirow{4}{*}{0.001}} &
%  150 & 0.6134 & 185.71MB \\
% \multicolumn{1}{c}{} &
%  100 & 0.6105 & 125.57MB \\
% \multicolumn{1}{c}{} &
%   50 & 0.5944 & 62.51MB \\
% \multicolumn{1}{c}{} &
%   10 & 0.5692 & 12.53MB \\
% \multicolumn{1}{c}{} &
%   1 & 0.5290 & 1.25MB\\

% \hline
% \end{tabular}
% % }
% \caption{Accuracy, storage requirement, communication throughout and FLOPs in ABNS stage in training with various density and pool size settings on VGG11 with CIFAR10 dataset. All cost measurements are for one device.}
% \label{tb:pool}
% \end{table}
